# Supplementary material for: Identify and Quantify Various Dissipation Mechanisms of Josephson Junction in Superconducting Circuits
Source: arXiv:2508.15174 ancillary file (2025-11-16)
Supplement: Supplementary file 1 [file supp_mat_v2_ax.pdf]

# Supplementary Material to “Identity and Quantify Various Dissipation Mechanisms of Josephson Junction in Superconducting Circuits”

Hao Deng,<sup>1,2,\*</sup> Huijuan Zhan,<sup>3</sup> Lijuan Hu,<sup>3</sup> Hui-Hai Zhao,<sup>4</sup> Ran Gao,<sup>3,5</sup> Kannan Lu,<sup>3,5</sup> Xizheng Ma,<sup>3</sup> Zhijun Song,<sup>6</sup> Fei Wang,<sup>3,5</sup> Tenghui Wang,<sup>3</sup> Feng Wu,<sup>4</sup> Tian Xia,<sup>7</sup> Gengyan Zhang,<sup>8</sup> Xiaohang Zhang,<sup>9</sup> and Chunqing Deng<sup>3,5,†</sup>

<sup>1</sup>*School of Physical Science and Technology, ShanghaiTech University, Shanghai 201210, China*

<sup>2</sup>*School of Information Science and Technology, ShanghaiTech University, Shanghai 201210, China*

<sup>3</sup>*Quantum Science Center of Guangdong-Hong Kong-Macao Greater Bay Area, Shenzhen 518045, China*

<sup>4</sup>*Zhongguancun Laboratory, Beijing, China*

<sup>5</sup>*Z-Axis Quantum*

<sup>6</sup>*Shanghai E-Matterwave Sci & Tech Co., Ltd., Shanghai 201100, China*

<sup>7</sup>*Huaxin Jushu Microelectronics Co., Ltd., Hangzhou, China*

<sup>8</sup>*Zhejiang Laboratory, Hangzhou 311100, China*

<sup>9</sup>*The Institute for Brain Research, Advanced Interfaces and Neurotechnologies, Shenzhen Medical Academy of Research and Translation, Shenzhen, 518100 China*

In this Supplementary Material, we present additional details of our work described in the main text, covering the design, the fabrication processes, the cryogenic measurement setups, the supplementary experimental data, and the relevant analyses.

## DESIGN

We design the co-planar waveguide (CPW) for the junction-embedded resonator (JER) with the core/gap width of  $2/25 \mu\text{m}$ . The characteristic impedance is  $\sim 113.2 \Omega$ . Through this way, we achieve relatively high effective lumped-element inductance of the transmission-line resonator at  $\sim 2 \text{ nH}$ . Meanwhile, we carefully design the area of Josephson junction (JJ) and limit its effective linear inductance (ELI), therefore, the total ELI of JJs ( $L_{\text{TJ}}$ ) does not exceed 15% of the effective lumped-element inductance of the remaining resonator. The value of  $L_{\text{TJ}}$  is deduced by the circuit model simulation. In the simulation, the embedded JJ is represented by a linear inductor. The inductance of the linear inductor, i.e.,  $L_{\text{TJ}}$ , is determined by matching the simulated frequencies of the 1st and 2nd harmonics with the measurement results. The opening for JJ in the middle of JER is  $50 \mu\text{m}$  long for all the devices (including the dummy-JJ JERs). More designed/characterized parameters of the devices are listed in Tab. S1.

## FABRICATION

200-nm thick,  $\alpha$ -phase tantalum film is deposited on the  $c$ -plane sapphire substrate (Suzhou RDMICRO Co. Ltd.) by sputtering (Labline, Kurt J. Lesker Company) with a 99.9999% purity target (H.C. Stark GmbH). Following the deposition, the geometry of CPW resonator is patterned by the direct-write-laser system (DWL 2000, Heidelberg Instrument GmbH), and finally transferred to the tantalum film through dry etching (LE0757, SPTS

Technologies Ltd.). The aluminum JJ is fabricated by the “Manhattan” method. We first pattern the geometry of JJ with e-beam lithography (JBX 8100FS, JOEL Inc.), then, implement the double-angle deposition and in-situ oxidation (JEB-D, AdNaNoTek Ltd.). The complete junction structure forms after the lift-off process.

## MEASUREMENT SETUPS

We perform the standard power-dependence measurement of resonator with the vector network analyzer (N5225B, Keysight Technologies Inc.). The samples are cooled down to  $\sim 15 \text{ mK}$  in a dilution refrigerator (LD400, Bluefors Oy). Fig. S1 shows the details of the channel configuration in the cryogenic environment.

## FREQUENCIES OF RESONATORS ON SAMPLE B

In Fig. S2, we demonstrate the analysis on the frequencies of the resonators on sample B. Consistent with the results of sample A, on sample B, the controlled devices (Ctrl. 1 and 2) and the dummy-JJ resonator shows slightly negative  $\Delta$  which is  $1/2 f_{2\text{H}} - f_{1\text{H}}$ . As a comparison, JER shows a clear dependence of  $\Delta$  on the number of JJ: with the increase of JJ number,  $\Delta$  increases. The extracted  $L_{\text{TJ}}$  through the circuit model simulation and the measured 1st- and 2nd-harmonic frequencies is close to the design target.

## NONLINEARITY OF JER AT HIGH PROBING POWER

Another approach to verify the involvement of JJ in JER is to check the nonlinearity of the 1st harmonic. It is expected that, the controlled devices and dummy-JJ JER should have no nonlinearity regardless the probing

| Sample | Device   | $f_{1H}$<br>(GHz) | $f_{2H}$<br>(GHz) | $\Gamma_{LP,1H}$<br>( $10^{-6}$ ) | $\Gamma_{LP,2H}$<br>( $10^{-6}$ ) | Resonator effective<br>lumped-element in-<br>ductance (nH) | $A_J$<br>( $\mu m^2$ ) | JJ<br>number | $L_{TJ}$<br>(nH) |
|--------|----------|-------------------|-------------------|-----------------------------------|-----------------------------------|------------------------------------------------------------|------------------------|--------------|------------------|
| A      | Ctrl. 1  | 6.079             | 12.142            | $1.51 \pm 0.05$                   | $1.28 \pm 0.03$                   | 1.88                                                       |                        |              |                  |
| A      | Ctrl. 2  | 6.024             | 12.033            | $1.32 \pm 0.03$                   | $1.46 \pm 0.04$                   | 1.90                                                       |                        |              |                  |
| A      | Dummy-JJ | 5.962             | 11.913            | $1.42 \pm 0.05$                   | $2.36 \pm 0.17$                   | 1.92                                                       |                        |              |                  |
| A      | L-JJ     | 5.851             | 11.804            | $3.01 \pm 0.13$                   | $2.86 \pm 0.12$                   | 1.94                                                       | 44.3                   | 2            | 0.08             |
| A      | M-JJ     | 5.731             | 11.685            | $2.24 \pm 0.12$                   | $3.08 \pm 0.12$                   | 1.96                                                       | 20.6                   | 2            | 0.19             |
| A      | S-JJ     | 5.619             | 11.571            | $1.93 \pm 0.03$                   | $2.82 \pm 0.17$                   | 1.98                                                       | 13.0                   | 2            | 0.29             |
| B      | Ctrl. 1  | 6.081             | 12.147            | $1.20 \pm 0.08$                   | $1.10 \pm 0.09$                   | 1.88                                                       |                        |              |                  |
| B      | Ctrl. 2  | 6.022             | 12.018            | $1.12 \pm 0.07$                   | $1.08 \pm 0.05$                   | 1.90                                                       |                        |              |                  |
| B      | Dummy-JJ | 5.964             | 11.917            | $1.24 \pm 0.05$                   | $1.91 \pm 0.17$                   | 1.92                                                       |                        |              |                  |
| B      | 2-JJ     | 5.844             | 11.789            | $2.54 \pm 0.37$                   | $2.97 \pm 0.06$                   | 1.94                                                       | 44.3                   | 2            | 0.08             |
| B      | 4-JJ     | 5.731             | 11.669            | $4.14 \pm 0.10$                   | $2.59 \pm 0.22$                   | 1.96                                                       | 44.3                   | 4            | 0.19             |

TABLE S1. Designed and characterized parameters of the resonators.  $f_{1H}$  and  $f_{2H}$  are measured frequencies of the 1st and 2nd harmonics, respectively.  $\Gamma_{LP,1H}$  and  $\Gamma_{LP,2H}$  are measured  $\Gamma_{LP}$ s of 1st and 2nd harmonics, respectively (i.e., the data points of Fig. 3(b) and 3(c) in the main text).  $A_J$  is the area of single JJ measured by the scanning electron microscope.  $L_{TJ}$  is the total ELI of JJs. The data of 6-JJ JER of sample B are not measurable because of its malfunction.

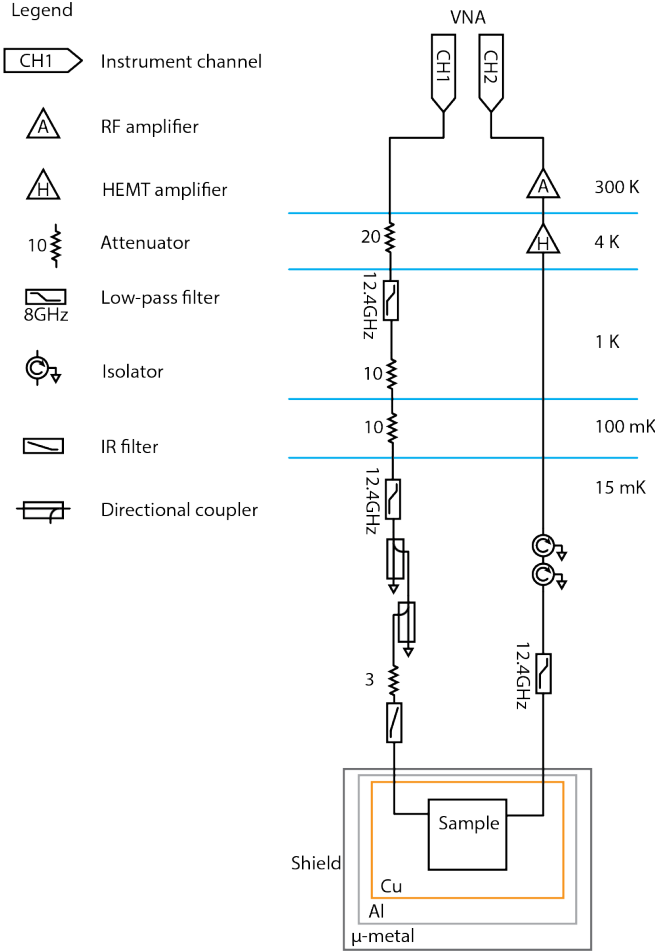

FIG. S1. Schematic of the measurement setup. The attenuations (in unit of dB) of the attenuators and cutoff frequencies of the low-pass filters are annotated beside the legends in the schematic. The coupling strength of the directional coupler is -20 dB.

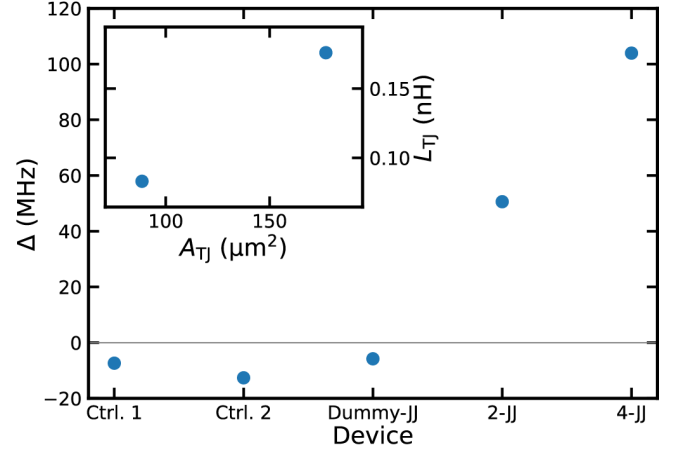

FIG. S2.  $\Delta$  (defined as  $1/2 f_{2H} - f_{1H}$ ) of all the resonators on sample B. About the x-axis, Ctrl. 1 and 2 represent 2 controlled devices which are normal resonators; Dummy-JJ, 2-JJ, and 4-JJ are the JERs containing dummy, 2, and 4 JJs, which are in the ascending order of ELI. The inset shows the extracted total ELI of JJs ( $L_{TJ}$ ) depending on the total junction area ( $A_{TJ}$ ). We are not able to acquire the data points of 6-JJ JER because of its malfunction.

power, but JERs with JJ embedded inside should have nonlinear behaviors in the high-power regime. Fig. S3 shows that, the nonlinearities of the resonators on both samples match the expectation.

With a close look on the data in Fig. S3, some subtle difference between the JERs of sample A and B could be noticed. For the JERs on sample A, the nonlinearity becomes stronger with the decrease of JJ area on 2 aspects: the critical power triggering nonlinearity decreases, and the drifting of  $f_{1H}$  becomes more significant. However, for the JERs on sample B, the drifting of  $f_{1H}$  becomes stronger with the increase of JJ number, but the criti-

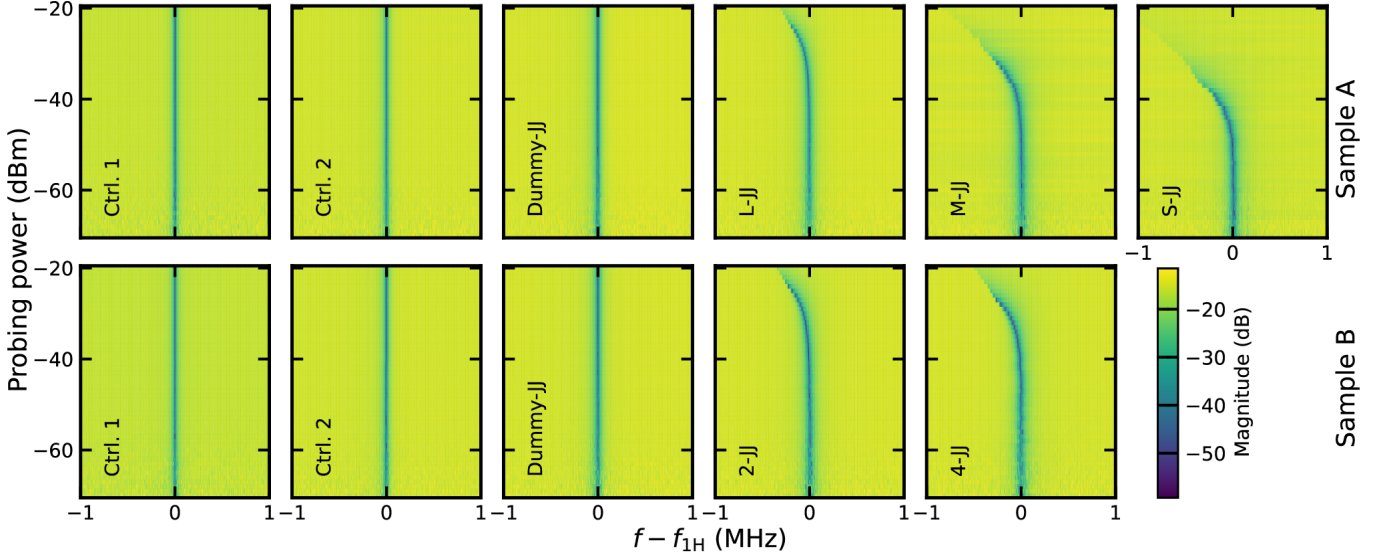

FIG. S3. Transmission signal magnitude of resonator depending on the probing frequency and power. The sub-figures in the 1st/2nd row shows the data of devices on sample A/B. The x-axis is the difference between the probing frequency and  $f_{1H}$ . The y-axis is the probing power at room-temperature stage.

cal power seems to be almost consistent ( $\sim 30$  dBm) for both 2- and 4-JJ JERs.

Such behaviors are consistent with the different ways to vary the JJs on sample A and sample B. In sample A, the JJ area is tuned. The critical current decreases when JJ area is reduced, and the nonlinearity of JJ increases. However, in sample B, the JJ area is fixed, so is the critical current. But the increase of JJ number in series adds more contributions of JJ to JER. Therefore, the nonlinearity of JER responding to the probing power also qualitatively confirmed that, in our samples, JJs involve in JERs as the design.

#### INDUCTIVE AND CAPACITIVE PARTICIPATION RATIO OF JJ IN JER

The inductive participation ratio of JJ ( $P_{TJ,L}$ ) is defined as the proportion of the inductive energy stored in ELI of all JJs ( $E_{TJ,L}$ ) among the full energy in JER ( $E_{CPW}$ ). As our discussions in the main text, if the inductive loss of ELI of JJ is significant, it is expected that the internal dissipation (i.e., 1st-harmonic dissipation rate of total JJ,  $\Gamma_{TJ,1H}$ ) should demonstrate a positive correlation with  $P_{TJ,L}$ . More than the qualitative discussion in the main text, we demonstrate a more quantitative analysis here.

More quantitative understanding on the voltage distribution along the transmission line of JER is necessary to deduce  $P_{TJ,L}$ . As what Fig. S4 shows, the amplitudes of the anti-node voltage of JER ( $V_{CPW}$ ) and the total voltage drop across JJ ( $V_{TJ}$ ) determines the energy stored in JER and JJ, respectively. With the circuit model and

the extracted  $L_{TJ}$  listed in Tab. S1, the ratio of these 2 voltages ( $V_{TJ}/V_{CPW}$ ) could be calculated. Then, We consider  $E_{TJ,L}$ :

$$\begin{aligned} E_{TJ,L} &= N \frac{1}{2} L_J I_J^2 = \frac{1}{2} L_{TJ} I_J^2 \\ &= \frac{1}{2} L_{TJ} \left| \frac{V_{TJ}}{j 2 \pi f_{1H} L_{TJ}} \right|^2 = \frac{1}{2} \frac{1}{(2 \pi f_{1H})^2} \frac{V_{TJ}^2}{L_{TJ}} \end{aligned} \quad (S1)$$

where  $N$  is the number of JJ.  $L_J$  is ELI of single JJ, therefore, for  $N$  JJs in series,  $L_{TJ} = N L_J$ .  $I_J$  is the current flowing through JJ.

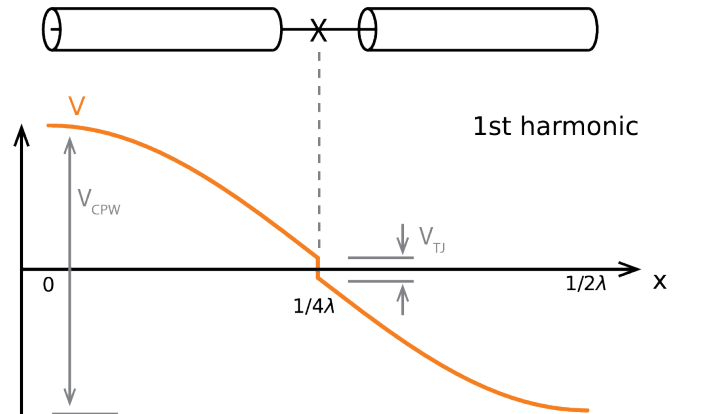

FIG. S4. Schematic of the JER and the voltage distribution of the 1st harmonic. The orange curve indicates the voltage distribution along the JER.  $V_{CPW}$  is the amplitude of voltage at the voltage anti-node.  $V_{TJ}$  is the total voltage drop across JJ. Note that  $V_{CPW}$  and  $V_{TJ}$  are not plotted in scale.

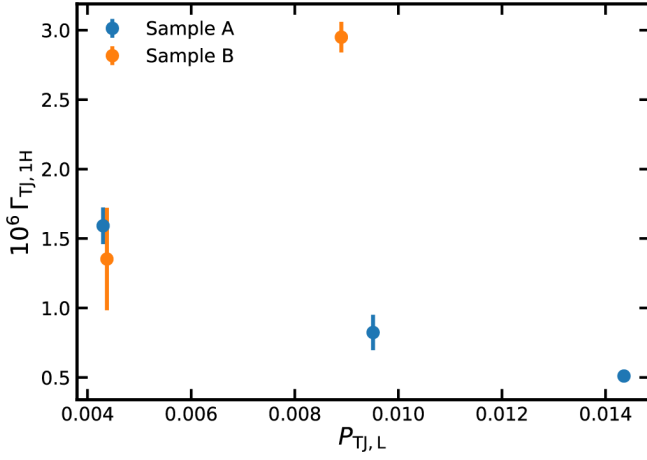FIG. S5. Dependence of  $\Gamma_{TJ,1H}$  on  $P_{TJ,L}$ .

For  $E_{CPW}$ , by assuming that  $E_{TJ,L}$  contains only a small part of energy:

$$E_{CPW} \simeq \frac{1}{2} C_{CPW} V_{CPW}^2 \quad (S2)$$

where  $C_{CPW}$  is the effective lumped-element capacitance of the transmission-line resonator, which could be deduced by the circuit model simulation with the measured resonance frequencies. Finally, we have the inductive participation ratio of **JJ**:

$$P_{TJ,L} = \frac{E_{TJ,L}}{E_{CPW}} = \frac{1}{(2\pi f_{1H})^2} \frac{1}{C_{CPW} L_{TJ}} \left( \frac{V_{TJ}}{V_{CPW}} \right)^2 \quad (S3)$$

Fig. S5 shows the dependence of  $\Gamma_{TJ,1H}$  on  $P_{TJ,L}$ . First, we notice that, for the **JER** with the largest  $P_{TJ,L}$  (i.e., S-JJ **JER** of sample A),  $P_{TJ,L}$  is  $\sim 1.4\%$ . This result indicates that,  $E_{TJ,L}$  indeed takes only a small part of  $E_{CPW}$ , and our deduction of  $P_{TJ,L}$  is self-consistent. Also, such low  $P_{TJ,L}$  confirms again that, the embedded **JJ** is a perturbation to the remaining transmission-line resonator, which matches our design target. Then, it is clear that, the data points of different samples show different dependence on  $P_{TJ,L}$ . Particularly, for the **JER** on sample A,  $\Gamma_{TJ,1H}$  decreases with the increase of  $P_{TJ,L}$ , which is a negative correlation. Therefore,  $P_{TJ,L}$  seems not a universal parameter describing the behaviors of  $\Gamma_{TJ,1H}$  of both samples.

In **JJ**, the aluminum/aluminum oxide/aluminum structure forms a capacitor. If this capacitor has dielectric loss, when finite  $V_{TJ}$  is applied on **JJs**, dissipation is expected to happen. To verify this hypothesis, we can check the dependence of  $\Gamma_{TJ,1H}$  on the capacitive participation ratio of **JJ** ( $P_{TJ,C}$ ), which is the proportion of the capacitive energy of **JJ** ( $E_{TJ,C}$ ) among  $E_{CPW}$ . We consider  $E_{TJ,C}$ :

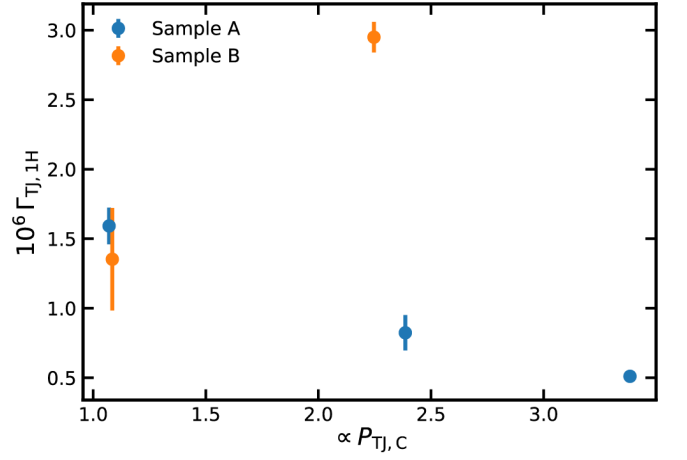FIG. S6. Dependence of  $\Gamma_{TJ,1H}$  on  $P_{TJ,C}$ .

$$E_{TJ,C} = N \frac{1}{2} C_J V_J^2 = N \frac{1}{2} C_J \left( \frac{V_{TJ}}{N} \right)^2 \quad (S4)$$

where  $C_J$  is the capacitance of single **JJ**, and  $V_J$  is the voltage across single **JJ**. The exact value of  $C_J$  requires complete information of the **JJ** barrier such as barrier thickness and the dielectric constant, which are difficult to characterize experimentally. However, to verify the correlation between  $\Gamma_{TJ,1H}$  and  $P_{TJ,C}$ , the scaling but not precise value of  $P_{TJ,C}$  is sufficient. Therefore, assuming that **JJ** capacitor is similar to the parallel plate capacitor:

$$E_{TJ,C} \propto N \frac{1}{2} A_J \left( \frac{V_{TJ}}{N} \right)^2 = \frac{1}{2} A_{TJ} \left( \frac{V_{TJ}}{N} \right)^2 \quad (S5)$$

where  $A_J$  is the area of single **JJ**, so that  $A_{TJ} = N A_J$ . With Eq. S2, we have:

$$P_{TJ,C} = \frac{E_{TJ,C}}{E_{CPW}} \propto \frac{1}{N^2} \frac{A_{TJ}}{C_{CPW}} \left( \frac{V_{TJ}}{V_{CPW}} \right)^2 \quad (S6)$$

We demonstrate the dependence of  $\Gamma_{TJ,1H}$  on  $P_{TJ,C}$  in Fig. S6. Similar to the results of  $P_{TJ,L}$ ,  $P_{TJ,C}$  fails to describe the behaviors of both samples universally. However, we would like to point out that, the results showed by Fig. S6 does not exclude the contributions of defects inside the barrier to the internal dissipation of **JJ**. Our analysis implies that, rather than the dielectric loss of a conventional, classical capacitor, these defects inside **JJ** barrier perhaps play their roles in the internal dissipation through an unexpected way, which is of great interest to study.

---

\* denghao1@shanghaitech.edu.cn

<sup>†</sup> [dengchunqing@quantumsc.cn](mailto:dengchunqing@quantumsc.cn)
